# Supplementary material for: Tetris is Hard, Even to Approximate
Source: arXiv:cs/0210020 source file (2002-10-21)
Supplement: Supplementary file 1 [file rtick.tex]

\subsubsection{Right-Ticks}

\begin{proposition}
  \mylabel{prop:ls-rtick}  
  There is no valid move for $\tLS$ in a right-tick bucket.
\end{proposition}
\begin{proof}
  The possible configurations are the following, since the $\tLS$
  cannot pass the tick:
  \begin{center}
    \input{figures/lsrtick}
  \end{center}
  (The second configuration has the $\tLS$ in the $i$th-highest notch.)
  
  All four have holes.
\end{proof}

\begin{proposition}
  \mylabel{prop:sqsq-rtick}  
  There is no valid move for $\tup{\tSq,\tSq}$ in a right-tick bucket.
\end{proposition}
\begin{proof}
  The first $\tSq$ cannot pass the tick, so the possible
  configurations are the following:
  \begin{center}
    \ifredraw
\begin{tabular}{llll}
  \begin{block}{5}{12}
    \column{1}{12}
    \piece{\LGr[lightgray]}2{0}
    \piece{\Sq[lightgray]}1{2}
    \piece{\Sq[red]}04
  \end{block} 
&
  \begin{block}{5}{12}
    \column{1}{12}
    \piece{\LGr[lightgray]}2{0}
    \piece{\Sq[lightgray]}1{2}
    \piece{\Sq[green]}14
  \end{block} 
\\\\
\end{tabular}
\else
\includegraphics{figures/rtick/sqrtick.epsi.clean}
\fi
%%% Local Variables: 
%%% mode: latex
%%% TeX-master: "../tetris"
%%% End: 

  \end{center}
  The first has a hole; the second is potentially valid.
  
  The results of placing the second $\tSq$, though, are as follows:
  \begin{center}
    \ifredraw
\includegraphics{figures/rtick/sqsqrtick.epsi.clean}
\begin{tabular}{llll}
  \begin{block}{5}{12}
    \column{1}{12}
    \piece{\LGr[lightgray]}2{0}
    \piece{\Sq[lightgray]}1{2}
    \piece{\Sq[green]}14
    \piece{\Sq[red]}06
  \end{block} 
&
  \begin{block}{5}{12}
    \column{1}{12}
    \piece{\LGr[lightgray]}2{0}
    \piece{\Sq[lightgray]}1{2}
    \piece{\Sq[green]}14
    \piece{\Sq[red]}16
  \end{block} 
\\\\
\end{tabular}
\else
\includegraphics{figures/rtick/sqsqrtick.epsi.clean}
\fi
%%% Local Variables: 
%%% mode: latex
%%% TeX-master: "../tetris"
%%% End: 

  \end{center}
  Both have holes, so there is no valid move sequence for $\tup{\tSq,
    \tSq}$.
\end{proof}

\begin{proposition}
  \mylabel{prop:lg-rtick}  
  If $\tLG$ is placed validly in a right-tick bucket, the result is a
  ($\tLG$-RT-$i$) for some $i$.
\end{proposition}
\begin{proof}
  The following configurations are possible with the $\tLG$ placed
  vertically:
  \begin{center}
    \ifredraw
\begin{tabular}{llllllllllllll}
\begin{block}{5}{16}
    \column{1}{16}
    \piece{\LGr[lightgray]}2{0}
    \piece{\Sq[lightgray]}1{2}
  \piece{\LGd[red]}02
\end{block}
&
\begin{block}{5}{16}
    \column{1}{16}
    \piece{\LGr[lightgray]}2{0}
    \piece{\Sq[lightgray]}1{2}
  \piece{\LGd[red]}14
\end{block}
&
\begin{block}{5}{16}
    \column{1}{16}
    \piece{\LGr[lightgray]}2{0}
    \piece{\Sq[lightgray]}1{2}
  \piece{\LGd[red]}2{10}
\end{block}
&
\begin{block}{5}{16}
    \column{1}{16}
    \piece{\LGr[lightgray]}2{0}
    \piece{\Sq[lightgray]}1{2}
  \piece{\LGu[red]}04
\end{block}
&
\begin{block}{5}{16}
    \column{1}{16}
    \piece{\LGr[lightgray]}2{0}
    \piece{\Sq[lightgray]}1{2}
  \piece{\LGu[red]}14
\end{block}
&
\begin{block}{5}{16}
    \column{1}{16}
    \piece{\LGr[lightgray]}2{0}
    \piece{\Sq[lightgray]}1{2}
    \piece{\LGl[red]}04
\end{block}
&
\begin{block}{5}{16}
    \column{1}{16}
    \piece{\LGr[lightgray]}2{0}
    \piece{\Sq[lightgray]}1{2}
  \piece{\LGr[red]}04
\end{block}
&
\begin{block}{5}{16}
    \column{1}{16}
    \piece{\LGr[lightgray]}2{0}
    \piece{\Sq[lightgray]}1{2}
    \piece{\LGr[red]}1{12}
\end{block}
&
\begin{block}{5}{16}
    \column{1}{16}
    \piece{\LGr[lightgray]}2{0}
    \piece{\Sq[lightgray]}1{2}
    \piece{\LGr[green]}2{12}
\end{block}
\\\\
\end{tabular}
\else
\includegraphics{figures/rtick/lgrtick1.epsi.clean}
\fi
%%% Local Variables: 
%%% mode: latex
%%% TeX-master: "../tetris"
%%% End: 

  \end{center}
  (The $i$th-highest notch is partially filled in the third, eighth,
  and ninth configurations, for any $i > 0$.)
  
  Of these, there is a hole is all but the last, which is a
  ($\tLG$-RT-$i$).
\end{proof}

\begin{proposition}
  \mylabel{prop:ls-rtick-notched}  
  There is no valid placement of $\tLS$ in ($\tLG$-RT-$i$) for any
  $i$.
\end{proposition}
\begin{proof}
  The following configurations are possible:
  \begin{center}
    \ifredraw
\begin{tabular}{llllllllllllll}
\begin{block}{5}{20}
    \column{1}{20}
    \piece{\LGr[lightgray]}2{0}
    \piece{\Sq[lightgray]}1{2}
    \piece{\LGr[lightgray]}2{12}
    \piece{\LSd[red]}03
\end{block}
&
\begin{block}{5}{20}
    \column{1}{20}
    \piece{\LGr[lightgray]}2{0}
    \piece{\Sq[lightgray]}1{2}
    \piece{\LGr[lightgray]}2{12}
    \piece{\LSd[red]}14
\end{block}
&
\begin{block}{5}{20}
    \column{1}{20}
    \piece{\LGr[lightgray]}2{0}
    \piece{\Sq[lightgray]}1{2}
    \piece{\LGr[lightgray]}2{12}
    \piece{\LSd[yellow]}1{13}
\end{block}
&
\begin{block}{5}{20}
    \column{1}{20}
    \piece{\LGr[lightgray]}2{0}
    \piece{\Sq[lightgray]}1{2}
    \piece{\LGr[lightgray]}2{12}
    \piece{\LSl[red]}04
\end{block}
&
\begin{block}{5}{20}
    \column{1}{20}
    \piece{\LGr[lightgray]}2{0}
    \piece{\Sq[lightgray]}1{2}
    \piece{\LGr[lightgray]}2{12}
    \piece{\LSl[red]}0{14}
\end{block}
&
\begin{block}{5}{20}
    \column{1}{20}
    \piece{\LGr[lightgray]}2{0}
    \piece{\Sq[lightgray]}1{2}
    \piece{\LGr[lightgray]}2{12}
    \piece{\LSl[red]}1{18}
\end{block}
\\\\
\end{tabular}
\else
\includegraphics{figures/rtick/lsrticknotch.epsi.clean}
\fi

%%% Local Variables: 
%%% mode: latex
%%% TeX-master: "../tetris"
%%% End: 

  \end{center}
  (Initially the $i$th-highest notch is filled with the $\tLG$.  The
  fifth denotes the $\tLS$ in the $j$th notch, for any $j \not= i$.
  The second and fourth configurations are blocked if $i=1$.)
  
  Of these, there is a hole is all but the third.  The last is a
  \bl{\alpha} for some $\alpha \not\equiv 0 ~(\mod 4)$, since the
  unfilled segments of the second and third columns differ in height
  by one.
\end{proof}

%%% Local Variables: 
%%% mode: latex
%%% TeX-master: "tetris"
%%% End: 
