# Supplementary material for: Tetris is Hard, Even to Approximate
Source: arXiv:cs/0210020 source file (2002-10-21)
Supplement: Supplementary file 2 [file appbadconfigs.tex]

\begin{theorem}  \label{thm:inst-bad}
  The following configurations are invalid, even under instantaneous
  rotation rules:
  \begin{CompactEnumerate}
  \item holes.  \label{holes-bad}
  \item a spurned notch, if the spurning occurs in the second column.
  \item an \bl{\alpha}, in any of the following cases:
    \begin{CompactEnumerate}
    \item in the row underneath a notch, we have 011, 110, or 111.
    \item the two-column high configuration [0;1] occurs in the either
      the second or third column with the bottom unfilled square in
      the first, second, or third row below a notch.
    \item a \bl{1} in a row without a notch.
    \item any \bl{2}.
    \item any situation in which the second and third columns are
      ragged on one side (mod 4).
    \end{CompactEnumerate}
  \end{CompactEnumerate}
\end{theorem}

%%% Local Variables: 
%%% mode: latex
%%% TeX-master: "tetris"
%%% End: 
